# Supplementary material for: SVD-LLM V2: Optimizing Singular Value Truncation for Large Language Model Compression
Source: arXiv:2503.12340 source file (2025-03-16)
Supplement: Supplementary file 1 [file 6_Appendix.tex]

\section{Appendix}
\label{sec:appendix}
\subsection{Compression Speed Analysis}
\label{appendix:compression_speed_analysis}
Apart from measuring the compressed LLMs' performance, we also evaluate the compression speed of \sysname and the baselines, including ASVD and SVD-LLM. Specifically, we measured the A100 GPU hours used for \sysname and the baseline methods when compressing LLaMA-7B under 20\% compression ratio. The results show that ASVD takes about 5.5 GPU hours, SVD-LLM takes about 15 minutes, while \sysname takes about 1.5 GPU hours to run the compression. Since \sysname not only requires computing the whitening matrices, which consumes the majority of time in SVD-LLM, but also needs to run its own key modules during compression, it is expected to consume longer time than SVD-LLM. However, it is still faster than ASVD, indicating that its compression time is still acceptable for post-training LLM compression. Moreover, our time breakdown analysis shows that the heterogeneous compression ratio allocation only requires 2 minutes, while the loss-minimized weight truncation takes up almost all 1.5 hours. Although this module is time-consuming, it deserves the time cost, as it helps \sysname significantly reduce its truncation loss during the SVD compression.

\subsection{Optimization Details}
\label{appendix:optimization_details}
In our experiments, we use the L-BFGS~\citep{Nash1991ANS} algorithm to perform optimization in loss-minimized weight truncation due to its benefits for fast convergence, especially when dealing with large-scale problems. We set the learning rate to 0.01 and the maximum iteration to 40. Our empirical results show that the loss drops rapidly and often converges in 20 iterations. Therefore, the time consumed to perform this optimization is still acceptable. As mentioned in~\cref{appendix:compression_speed_analysis}, it only takes about 1.5 hours to optimize all weight matrices in LLaMA-7B, which also meets our initial goal of designing an efficient and practical way to minimize truncation loss.
